# Supplementary material for: Multi-objective Explanations of GNN Predictions
Source: arXiv:2111.14651 source file (2021-11-29)
Supplement: Supplementary file 1 [file supp.tex]

\section{Supplementary}
\titlespacing*{\section}{0pt}{1.1\baselineskip}{\baselineskip}

\subsection{DFS Algorithm for subgraph enumeration}
\begin{algorithm}[h]
\small
	\caption{GNNCFE}
	\label{algo:GNNEXPAlg}
	\LinesNumbered
	\KwIn{Graph $G=(V,E)$, target GNN model, a target node $v_i \in V$ to be explained, maximum subgraph size $C$, search diameter $D$, number of explanations diversity $K$}
	\KwOut{Top $p\%$ explanations $(G_i,\tilde{G}_i)$ for $v_i$}
	\SetKwFunction{FMain}{GNNCFE}
    \SetKwProg{Fn}{Function}{:}{}
    \Fn{\FMain{}}{
    $S_s$ = DFSEnumerate$(G,\{v_i\},v_i,\emptyset)$ \; 
    \ForEach{$S \in S_s$}{
        \ForEach{$v_j \in S$}{
        $\mu(v_j; v_i, S) = \nu(S, v_i) - \nu(S \setminus \{v_j\}, v_i)$}
    }
    \textbf{Return} Top $p\%$ explanations $\mu(v_j; v_i, S)$ for $v_i$
    }
    \textbf{End Function}\;
	\SetKwFunction{FMain}{DFSEnumerate}
    \SetKwProg{Fn}{Function}{:}{}
    \Fn{\FMain{G, Sub, v, Forbidden}}{
    // $Sub$: current subgraph;  $v$: current node to explore. \; 
     \ForEach{u $\in \mathcal{N}(v)$}{
        \uIf{$(v,u) \not\in$ Fobidden \textnormal{and} $len(Sub)<C$ \textnormal{and} $u$ less than $D$-hops away from $v_i$
        }
            {DFSEnumerate($G,Sub\cup\{(v,u)\},u,Forbidden$)\; 
            $Forbidden \longleftarrow Forbidden \cup\{(v,u)\}$ \; }
        }
        \ForEach{m $\in$ $Sub \setminus \{v\}$}{ // \textit{expand from other variables.}
        DFSEnumerate($G,Sub,m,Forbidden$)\;
        }
        % \textbf{print Sub}
    \textbf{Return} $Sub$ \\
    }
    \textbf{End Function}\;
\end{algorithm}
\subsection{Reproducibility checklist}
\begin{table}[h]
    \scriptsize
    \centering
    \begin{tabular}{c|c|c|c|c|c}
    \toprule
    \textbf{Datasets} & \textbf{Classes} & \textbf{Nodes} & \textbf{Edges} & \textbf{Edge/Node} & \textbf{Features}\\
    \midrule
    \textbf{Cora} & 7 & 2,708 & 10,556 & 3.90 & 1,433\\
    \textbf{Citeseer} & 6 & 3,321 & 9,196 & 2.78 & 3,703\\
    \textbf{PubMed} & 3 & 1,9717 & 44,324 & 2.24 & 500\\
    \midrule
    \textbf{Musae-F} & 4 & 2,2470 & 342,004 & 15.22 & 4,714\\
    \textbf{Musae--G} & 2 & 37,700 & 578,006 & 15.33 & 4,005\\
    \midrule
    \textbf{Amazon-C} & 4 & 13,752 & 574,418 & 41.77 & 767\\
    \textbf{Amazon-P} & 6 & 7,650 & 287,326 & 37.56 & 745\\
    \midrule
    \textbf{Coauthor-C} & 13 & 18,333 & 327,576 & 17.87 & 6,805\\
    \textbf{Coauthor-P} & 2 & 34,493 & 991,848 & 28.76 & 8,415\\
    \bottomrule
    \end{tabular}
     \caption{Nine networks from four application domains.}
     \label{tab:datasets}
\end{table}

\begin{table}[t]
\caption{\small Overall performance (the higher the simulatability or the counterfactual relevance is, the better).
The worst performances are underlined.
The simulatability is how often the subgraphs can preserve the prediction outcomes of the original GNN.
The counterfactual relevance is the absolute value of the change in probability of the prediction
outcomes of the GNN.
}
\centering
\scriptsize
%\small
\begin{tabular}{c
                ||@{\hspace*{1mm}}c
                @{\hspace*{1mm}}c
                @{\hspace*{1mm}}c
                @{\hspace*{1mm}}c
                @{\hspace*{1mm}}c
                @{\hspace*{1mm}}c
                @{\hspace*{1mm}}c 
                @{\hspace*{1mm}}c 
                }
\toprule
    \multirow{2}{*}{\textbf{Datasets}} &
    \multicolumn{7}{c}{\textbf{Simulatability}} \\
%  \cline{2-15}

& 
\textbf{Random} & 
\textbf{Embedding} & 
\textbf{Gradient} & 
\textbf{GAT} & 
\textbf{GNNExplainer} & 
\textbf{Shapley} & 
\textbf{GNNCFE}
\\

\midrule
Cora
& \makecell[c]{0.883}
& \makecell[c]{0.863}
& \makecell[c]{\underline{0.692}}
& \makecell[c]{0.869}
& \makecell[c]{0.881}
& \makecell[c]{0.912}
& \makecell[c]{\textbf{0.940}}
\\

Citeseer
& \makecell[c]{0.902}
& \makecell[c]{0.899}
& \makecell[c]{\underline{0.861}}
& \makecell[c]{0.904}
& \makecell[c]{0.894}
& \makecell[c]{0.928}
& \makecell[c]{\textbf{0.934}}
\\

PubMed
& \makecell[c]{0.926}
& \makecell[c]{0.908}
& \makecell[c]{\underline{0.682}}
& \makecell[c]{0.917}
& \makecell[c]{0.921}
& \makecell[c]{0.938}
& \makecell[c]{\textbf{0.978}}
\\

\midrule

Musae-F
& \makecell[c]{0.715}
& \makecell[c]{\underline{0.699}}
& \makecell[c]{0.709}
& \makecell[c]{0.742}
& \makecell[c]{0.744}
& \makecell[c]{0.745}
& \makecell[c]{\textbf{0.958}}
\\

Musae-G
& \makecell[c]{0.924}
& \makecell[c]{0.936}
& \makecell[c]{\underline{0.868}}
& \makecell[c]{0.924}
& \makecell[c]{0.896}
& \makecell[c]{0.926}
& \makecell[c]{\textbf{0.946}}
\\

\midrule
Amazon-C
& \makecell[c]{0.841}
& \makecell[c]{0.837}
& \makecell[c]{\underline{0.522}}
& \makecell[c]{0.843}
& \makecell[c]{0.830}
& \makecell[c]{0.906}
& \makecell[c]{\textbf{0.919}}
\\

Amazon-P
& \makecell[c]{0.851}
& \makecell[c]{0.837}
& \makecell[c]{\underline{0.630}}
& \makecell[c]{0.843}
& \makecell[c]{0.821}
& \makecell[c]{0.906}
& \makecell[c]{\textbf{0.921}}
\\

\midrule
Coauthor-C
& \makecell[c]{0.903}
& \makecell[c]{0.902}
& \makecell[c]{\underline{0.617}}
& \makecell[c]{0.895}
& \makecell[c]{0.896}
& \makecell[c]{0.925}
& \makecell[c]{\textbf{0.955}}
\\

Coauthor-P
& \makecell[c]{0.944}
& \makecell[c]{0.934}
& \makecell[c]{\underline{0.710}}
& \makecell[c]{0.915}
& \makecell[c]{0.932}
& \makecell[c]{0.942}
& \makecell[c]{\textbf{0.962}}
\\
% \hline
\bottomrule
\end{tabular}

\begin{tabular}{c
                ||@{\hspace*{1mm}}c
                @{\hspace*{1mm}}c
                @{\hspace*{1mm}}c
                @{\hspace*{1mm}}c
                @{\hspace*{1mm}}c
                @{\hspace*{1mm}}c
                @{\hspace*{1mm}}c 
                }
% \begin{tabular}{c||c|c|c|c||cccccccc}
\toprule
    \multirow{2}{*}{\textbf{Datasets}} &
    \multicolumn{7}{c}{\textbf{Counterfactual Relevance}} \\%\hline
& 
\textbf{Random} & 
\textbf{Embedding} & 
\textbf{Gradient} & 
\textbf{GAT} & 
\textbf{GNNExplainer} & 
\textbf{Shapley} & 
\textbf{GNNCFE}
\\

\midrule
Cora
& \makecell[c]{0.141}
& \makecell[c]{0.168}
& \makecell[c]{0.173}
& \makecell[c]{\underline{0.131}}
& \makecell[c]{0.138}
& \makecell[c]{0.204}
& \makecell[c]{\textbf{0.228}}
\\

Citeseer
& \makecell[c]{\underline{0.085}}
& \makecell[c]{0.091}
& \makecell[c]{0.090}
& \makecell[c]{0.086}
& \makecell[c]{0.086}
& \makecell[c]{0.108}
& \makecell[c]{\textbf{0.113}}
\\

PubMed
& \makecell[c]{0.107}
& \makecell[c]{0.124}
& \makecell[c]{0.166}
& \makecell[c]{0.111}
& \makecell[c]{\underline{0.101}}
& \makecell[c]{0.162}
& \makecell[c]{\textbf{0.185}}
\\

\midrule

Musae-F
& \makecell[c]{0.221}
& \makecell[c]{0.238}
& \makecell[c]{0.259}
& \makecell[c]{0.195}
& \makecell[c]{\underline{0.194}}
& \makecell[c]{0.304}
& \makecell[c]{\textbf{0.307}}
\\

Musae-G
& \makecell[c]{0.096}
& \makecell[c]{0.099}
& \makecell[c]{0.162}
& \makecell[c]{\underline{0.094}}
& \makecell[c]{0.104}
& \makecell[c]{0.156}
& \makecell[c]{\textbf{0.164}}
\\

\midrule
Amazon-C
& \makecell[c]{\underline{0.071}}
& \makecell[c]{0.078}
& \makecell[c]{0.147}
& \makecell[c]{0.072}
& \makecell[c]{0.075}
& \makecell[c]{0.124}
& \makecell[c]{\textbf{0.169}}
\\

Amazon-P
& \makecell[c]{0.079}
& \makecell[c]{0.087}
& \makecell[c]{0.135}
& \makecell[c]{0.077}
& \makecell[c]{\underline{0.072}}
& \makecell[c]{0.124}
& \makecell[c]{\textbf{0.159}}
\\

\midrule
Coauthor-C
& \makecell[c]{\underline{0.107}}
& \makecell[c]{0.119}
& \makecell[c]{0.184}
& \makecell[c]{0.116}
& \makecell[c]{0.113}
& \makecell[c]{0.183}
& \makecell[c]{\textbf{0.209}}
\\

Coauthor-P
& \makecell[c]{0.088}
& \makecell[c]{0.096}
& \makecell[c]{0.142}
& \makecell[c]{\underline{0.080}}
& \makecell[c]{0.093}
& \makecell[c]{0.168}
& \makecell[c]{\textbf{0.173}}
\\
\bottomrule
\end{tabular}

\label{tab:overall_}
\end{table}

\subsubsection{Datasets and setups}
We drew real-word datasets from four applications for the node classification task.
% of GNNs.
The statistics of the datasets are shown in Table \ref{tab:datasets}.
More details:
\begin{itemize}[leftmargin=*]
    \item 
In citation networks (Citeseer, Cora, PubMed)~\cite{kipf2017gcn}, each paper has bag-of-words features, and the goal is to classify the research area of each paper.
% Firstly, in collective classification,
% the goal is to classify a paper in a citation network into one of the many research areas.
% Nodes represent papers and edges indicate the reference relationship,
% where the features of the nodes are the bag of words of the paper.
% We construct an GNN for each of the three citation networks (Citeseer, Cora, PubMed)~\cite{kipf2017gcn}.
\item
we adopt Musae-Facebook (Musae-F) and Musae-Github (Musae-G)~\cite{rozemberczki2019multi} from social networks.
Nodes in Musae-F (or Musae-G) represent official Facebook pages (or Github developers), and edges are mutual likes (or followers) between nodes.
Node features are extracted from site descriptions
(or developer's location, 
repositories starred, employer).
% Secondly, we adopt two types of social networks (Musae-Facebook and Musae-Github)~\cite{rozemberczki2019multi}.
% The former is a page-page graph of verified Facebook sites.
% Nodes represent official Facebook pages while the links are mutual likes between sites,
% where node features are extracted from the site descriptions that the page owners created to summarize the purpose of the site. % The latter is a large social network of GitHub developers.
% Nodes are developers who have starred at least 10 repositories and edges are mutual follower relationships between them. 
% The vertex features are extracted based on the location, 
% repositories starred, employer and e-mail address.
\item
Amazon-Computer (Amazon-C) and Amazon-Photo (Amazon-P)~\cite{shchur2018pitfalls} are segments of the Amazon co-purchase graph,
where nodes represent goods, edges indicate that two goods are frequently bought together, node features are bag-of-words encoded product reviews.
% , and class labels are given by the product category.
\item
Coauthor-Computer and Coauthor-Physics are co-authorship graphs based on the Microsoft Academic Graph from the KDD Cup 2016.
We represent authors as nodes,
that are connected by an edge if they co-authored a paper~\cite{shchur2018pitfalls}.
Node features represent paper keywords for each author’s papers.
% and class labels indicate most active fields of study for each author.
\end{itemize}
% We divide 50 percent of the nodes into training sets, 20 percent into validation sets, and the rest into test sets
% for all of the above datasets.
% we use training sets to train GNN model, 
% and validation sets and test sets to evaluate GNN model.
% Our experiment is carried out on the test sets.
We divide each dataset into three portions with ratio of \textit{training : validation : test = 50 : 20 : 30}.
The GNN is trained on the training set and
% with validation set tuning the performance.
all explanation methods are evaluated on the test portion.

\subsubsection{Experimental environment}
% 7.3 and 7.4
We ran
the experiments on a Linux system,
with two CPU with six cores and two 8G GPU.
The amount of memory is 252G.
The results are obtained on the CPU.
Versions of the software for the implementation:
Python (3.7.0),
Numpy (1.15.1),
Pytorch(1.3.1).
All random seeds are fixed at 42.
% \subsubsection{Metric}
% 7.5
% We adopt two metrics simulatability and counterfactual relevance,
% which is our goal is to optimize.
% The details can be found in main text.
% Another more intuitive metric is how often the subgraphs can preserve the prediction outcomes of the original GNN.
% The results can be found in Table \ref{tab:overall_}.
\subsubsection{Repeated experiments and Hyperparameters}
% 7.6 and 7.7 and 7.8 and 7.9
We adopt a Graph Convolutional Network(GCN) model \cite{kipf2017gcn} as the target model to be explained,
with two hidden layers ($L=2$)
each with dimension 16.
% The dimensions of the input and output layers are set to different values depending on the datasets.
The dimension of the input layer is equal to the feature dimension of the nodes,
and the dimension of the output layer is set to the number of classification categories.
We adopt the cross-entropy loss function and the Adam optimizer for training the target GNN model,
while the learning rate of the optimizer is set to be 0.01.
We set the maximal training iterations to 500.
%with early stop using the validation sets.
If the performance of the model on the test set does not get better, 
the training will be stopped and the model with the best performance will be fixed and saved.
% All GNN models used in the experiment are loaded with the parameters.

% The details and division of all the datasets are mentioned above and all of our experiments are carried out on the test set.
% The two metrics the experiment described above are selected,
% and the means of the two metrics across all target nodes are reported, with statistical significance based onat-tests is indicated.
% There are two parameters $D$ and $C$,
% where $D$ limits the search scope and $C$ limits the complexity of the explanations.

\begin{tcolorbox}
\footnotesize
\noindent\textbf{Survey begins}

Please answer the following questions before you proceed.
\begin{itemize}
    \item Have you taken any courses in data mining, AI, or machine learning?
    \item Are you working on research related to data mining, AI, or machine learning?
    \item Are you an undergraduate or a graduate?
\end{itemize}

Now, suppose you are working on a course project and need to read some papers.
You're searching for papers using a search engine.
The engine can do some reasoning about the areas that a paper belongs to, based on citation information, such as the area of the papers citing or cited by the paper.
To help you make the final paper selection,
the search engine also tells you the probabilities of the areas that the paper belongs to.
For example, if a paper cites many papers in ``data mining'', then it is quite likely that the paper should belong to the ``data mining'' area, although there is a non-zero probability that the paper is in the machine learning area.

The search engine will try to explain to you how these probabilities are computed so that you can be assured of the correctness of the search, or you can identify and report errors to the software engineers who implement the search engine.
Since there are many papers interconnected by the citation relationship, the search engine explains the results using a small part of the entire dataset, where the probabilities are computed to be as close to the results on the full graph as possible.
You may or may not find the computation on the smaller graph convincing.
% Here we present some cases for you to decide if the model's reasoning is convincing or not.

% To make the explanations easier to understand,
% the search engine also highlight
% the papers that contribute most to the target paper's probabilities.

\noindent\textbf{Training cases}

Here we will use concrete examples to show you the above concepts and the steps to take in this survey.
You will see two columns of figures.
The first column is a network that contains the paper returned by the search engine, labeled by ``X''.
The second column is the probabilities of the seven areas that the target paper can belong to, according to the search engine's computation.

In the first row,
the larger graph $G1$ contains all the papers 
connected by citation relationship, and the target paper is labeled with $X$,

The search engine adopts global graph information for joint reasoning to determine which area each paper belongs to.
The color of each paper depends on the area predicted by the search engine algorithm
and matches the colors in the histogram.
For example,
the probability of the target paper $X$ belonging to "Probability Methods" on the larger graph $G1$ is 0.48 and is colored red.

In the second row, 
$G2$ is a subgraph of $G1$ where the probability of the target paper $X$ is calculated.
For example,
the probability of the target paper $X$ of being a "Probability Methods" paper on the subgraph $G2$ is 0.47, which is
close to the probability 0.48 on $G1$.

% \end{tcolorbox}
% \begin{tcolorbox}
% \footnotesize
% \noindent\textbf{Survey continued}

In the third row, 
$G3$ removes paper or papers from $G2$,
and the dashed line represents the edge that connects the removed component and $G$3.
The removal of the paper will lead to a change in the predicted probabilities of the target paper $X$,
presented in the second column.
For example,
the removal of paper $B$ will change the area of paper $X$
from "Probability Methods" to "Case Based",
so dose paper $A$.
Multiple papers can be removed from $G$2.
Notice the coloring of the nodes may change when going from $G$2 to $G$3.

In the fourth row, 
the operation is similar to the third row,
while a different set of paper(s) is removed.
For example,
the removal of paper $D$ has little effect on the probabilities of the target paper $X$,
while paper $X$ still belongs to "Probability Methods".

Answer the following four questions:
\begin{itemize}
    \item (\textit{\textcolor{red}{Simulatability}}) How well do you think the second subgraph $G$2 is reproducing the prediction computed in the first graph $G$1. \textcolor{blue}{(1-very little,2-little,3-not sure,4-a little, 5-very well)}.
    \item (\textit{\textcolor{red}{Counterfactual}}) How much do you think the removed component in the third subgraph $G$3 causes the search engine to predict the class distribution in the second subgraph $G$2, had it not been removed? \textcolor{blue}{(1-very little,2-little,3-not sure,4-a little, 5-very much)}.
    \item (\textit{\textcolor{red}{Counterfactual}}) How much do you think the removed component in the forth subgraph $G$4 causes the search engine to predict the class distribution in the second subgraph $G$2, had it not been removed? \textcolor{blue}{(1-very little,2-little,3-not sure,4-a little, 5-very much)}.
    \item (\textit{\textcolor{red}{Adoption of the explanation}}) How much will you accept the search engine's computation of the probabilities, if they were computed on the second smaller subgraph $G$2 rather than the first larger subgraph $G$1? \textcolor{blue}{(1-very little, 2-little,3-not sure,4-a little, 5-very much)}.
\end{itemize}
\end{tcolorbox}
